# Supplementary material for: Boosting Text-to-Chart Retrieval through Training with Synthesized Semantic Insights
Source: arXiv:2505.10043 source file (2026-03-17)
Supplement: Supplementary file 1 [file 4-Comparison_to_Chartqa.tex]

1
